# Supplementary material for: SoK: Cross-Domain MEV
Source: arXiv:2308.04159 source file (2023-08-08)
Supplement: Supplementary file 1 [file appendix.tex]

Some research developments in this area are: 
\begin{enumerate}
    
    \item On The Quality Of Cryptocurrency Markets: Centralized Versus Decentralized Exchanges \url{https://arxiv.org/pdf/2112.07386.pdf}.
    \item An Empirical Study of Market Inefficiencies in Uniswap and SushiSwap \url{https://arxiv.org/pdf/2203.07774.pdf}. This paper shows that on-chain markets become efficient, and opporunities disappear.
    \item Blockchain Intra- and Interoperability \url{https://static1.squarespace.com/static/57af6f83893fc027c794e637/t/60d7b9c0e71eb125bdc7928d/1624750530252/32+2021+Lipton+Hardjono+Blockchain+Intra+and+Interoperability.pdf}. This paper tries to formalize the players... Moderately interesting, but not really. 
    \item Unity is Strength: A Formalization of Cross-Domain Maximal Extractable Value \url{https://arxiv.org/pdf/2112.01472.pdf}.
    \item ODOS: DEX/cross-chain??? aggregator. Provides optimal routing across DEXs\url{https://odos.xyz/} Cross Domain Arb tracker: \url{https://www.odos.xyz/arbitrage}.
   
    \item HOP Exchange. Cross shard DEX where the bridge is effectively an AMM with a common token, managed by a \textit{bonder}. This bonder skips the necessity to always communicate via the Layer 1 blockchain, in exchange for a fee. 
    \item deBridge. A cross-chain messaging bridge (including for bridging assets) \url{https://debridge.finance/}.
    \item WooFi: Cross chain DEX using CEX prices as an oracle. 
    \item A lot of protocols are using LayerZero's Stargate to relay messages interchain (at least Sushi and WooFi). The protocol requires a relayer and oracle to verify transactions have been committed on the source chain before executing on the destination chain. No proving is done on the destination chain, making these intermediaries centralized players. 
    \item Hashflow seem to be the largest active cross-chain DEX. Requires active MMs providing quotes for users, presumably owning tokens on both chains. \url{https://docs.hashflow.com/hashflow/product/bridgeless-cross-chain-swaps}.
    \item Chainge Finance appears to offer a cross-chain DEX aggregator, \textit{finding the best price available} \url{https://www.coindesk.com/sponsored-content/cross-chain-liquidity-aggregation-delivers-best-prices-and-unlimited-liquidity/}.
    \item Thorchain offers cross-chain swaps, but all transactions happen on the ThorChain (Cosmos).
    \item Dodo allows for cross-chain swaps, althought seems to involve active quoting. Very unclear where tokens are coming from. (using "decentralized price oracles").
    \item Nice article by Variant Fund  \url{https://variant.fund/articles/cross-chain-order-flow-auctions/}.  Interesting terms: \begin{itemize}
        \item New sources of network effects emerge for L2s, we could see L2s buy up significant portions of L1 blockspace in order to crowd out other L2s’ access.
        \item App layer projects could run builders, with the goal of minimizing fee extraction for users.
    \end{itemize} 
    \item Osmosis ProtoRev. The Osmosis chain seems to be executing cyclic arbitrage (albeit restricted to the osmosis chain). Improving cross-chain atomicity improves the democratization of cross chain MEV.   \url{https://osmosis.zone/blog/osmosis-protorev-by-skip-protocol-on-chain-app-directed-arbitrage}
    \item Volt Capital. Primers on MEV across chains, with some interesting links and thoughts on current directions in the space  \url{https://volt.capital/writing}
    \item Nice article by JCharbonneau on SUAVE \url{https://mirror.xyz/jon-dba.eth/NTg5FSq1o_YiL_KJrKBOsOkyeiNUPobvZUrLBGceagg}. Some highlights:\begin{enumerate}
        \item ...this means that SUAVE cannot guarantee atomic inclusion of X-chain transactions by itself. You need the proposers of respective chains to agree on atomic inclusion for that guarantee to be enforced.
        \item SUAVE can’t provide “technical X-domain atomicity” on its own, but it can provide “economic X-domain atomicity” in this sense from the user perspective (though the executor may get stuck holding the risk, at an increased fee).
    \end{enumerate}
    \item Cross Chain communication is \textbf{impossible} without a TTP \url{https://eprint.iacr.org/2019/1128.pdf}. This paper also does a good job at formalization of cross-chain messaging. 
    \item Thread by @bertcmiller on how holding inventory risk results in strict domination of profits, specifically for sandwiching on Ethereum in this case. I think this is a good advocation that this will be the end goal \url{https://twitter.com/bertcmiller/status/1656392881538744321}.
    \item Mekatech \url{https://meka.tech/zenith} is trying to build a sequencer for multiple blockchains . One of their protections is: \textit{If for any reason Zenith fails to propose a block within a strict time limit, then the code falls back to the normal block production behavior.} These lads also provided an estimate of cross-domain opportunities on Cosmos chains \url{https://meka.tech/writing/analysing-cross-chain-arbitrage-opportunities-for-atom-fee57867-4385-4ead-b19c-8db75a753226}.
    
\end{enumerate}

Uniswap has approximately $5\%$ TVL outside of Ethereum. Several links mention cross-domain MEV as a centralizing force. Validators may be creating blocks on multiple blockchains. What effect will this have? Are there any protocols that are more vulnerable to the effect of multi-chain control?

\subsection{}
\section{Ideas}

Introduce the idea of protocol specific chains/sequencers to synchronize protocols. There are watchers that send signals from bell-weather pools/off-chain markets, which update the price of smaller pools on other chains. The longer the time between synchronizations, the higher the fee?

The obvious cross-domain MEV is arbitrage. What other types of MEV are going to emerge?
\begin{enumerate}
    \item Multi-domain schedulers executing user-level extraction, such as front-running, back-running, etc. 
    \item Cross-chain oracle manipulation... Not so clear what the vector is here.
    \item Denial-of-service (ransom) attacks...
    \item Chains need to be conscious of the ratio of native assets to bridged assets. If a single player or group of players can access a set of bridged assets for cheaper than the native assets required to control those bridged assets (liquidate positions, manipulate price oracles) while monopolizing control of the chain (preventing other bridgers/arbers/validators from correcting protocol states).
\end{enumerate}

\subsection{Unisuaap}

The centralized sequencer replicates the liquidity of the corresponding pools in each underlying chain. Doing this without a single centralized sequencer seems impossible. 

Maybe there is an impossibility result here that technically, blockchains can't synchronize without a trusted super-layer.
In this regard, the best we can do is to ensure some level of economic synchronicity. Something like chain $A$ knows the transaction can be executed on chain $B$, and if the information is incorrect, the transaction on chain $B$ loses money.

Don't try to achieve a technical guarantee of inclusion on another chain, just an economic guarantee.

The hypothesis:

\begin{lemma}
    Consider an LP providing liquidity on $n$ different domains. If all domains can be update closer to real-time, the expected LVR reduces (I think it is quadratically dependent). 
\end{lemma}

\begin{lemma}
    Consider an LP providing liquidity on $n$ different domains. If all domains can be update closer to real-time, the expected LVR reduces (I think it is quadratically dependent). 
\end{lemma}

Cross-domain mainly focusing on L2s. Understand IBC. Cosmos is big, how?

try and build a cross domain block builder, understanding when you can build blocks at the same time, and what can you do with that power? IS there much value in knowing another chains mempool/upcoming blocks before it gets built. Can builders exchange this information?

Formalizing why stat arb. dominates cross-domain MEV, why people leg into CEX legs?
Can we internalize cross-domain value extraction? Is it Binance agnostic?
Auctioning order-flow across domains, what exists? Are there improvements?
Consider block-space futures market, what does it mean for cross-domain MEV?

One statement is to talk cefi-defi arbers
- We want to internalize that value for our users, what can we do?
	- 1. an order-splitting protocol across liquidity pools across domains
	- 2. an auction that sells orderflow where you offload the work of finding liquidity pools to searchers
- Settle on a particular solution \& why, maybe quantifying the improvement for users, even a lower bound
- Reflect on some of the assumptions
	- what if Binance disappears? does that change anything?

\subsection{Intuition behind why CEX plays dominant part in arbitrage}

The world can be seen as $n$ different sources of liquidity, with CEX being the only continuous-time source of liquidity. In that sense, the instantaneous price of a CEX contains all available price information about all other $n-1$ DEXs. Each of the other $n-1$ sources are stale to the price information of the CEX. Every time an order meaningfully impacts the underlying price of a swap, this information is immediately sent to the CEX, in the form of an (implied) arbitrage between the informed source, and the CEX. 

Provide an example of the payoff of executing both legs against each other (with time delay), vs. executing both legs vs. CEX price. Profit should be approximately the same, minus CEX fees and probability of executing second leg. 

\begin{example}
    \normalfont
    Consider 2 DEXs $D_1$ and $D_2$ creating an arbitrage opportunity $A$ against both each other, and individually against the CEX $A_1$, $A_2$, with $A_1+A_2\leq A$. WLOG, let $A_1, A_2>0$. Given $A_1$ and $A_2$ are positive, they have offsetting effects on the spot price, with the external market price unaffected by the existence of the opportunities. After $A_1$, there will be some impact in the market, making $A_2$ greater conditioned on $A_1$ (the CEX has been moved against the DEX order/market creating $A_2$). Assume there is another searcher with the capability to extract $A_2$. The bid to extract 
\end{example}

\begin{example}
    \normalfont
    Consider 2 DEXs $D_1$ and $D_2$ creating an arbitrage opportunity $A$ against both each other, and individually against the CEX $A_1$, $A_2$, with $A_1+A_2\leq A$. Due to execution costs, we can make this less than or equal strict, with $A_1+A_2=A-(e_1+e_2)$, where $e_1,\ e_2>0$ are the costs to execute the centralized leg of both arbitrage opportunities. Why would people choose to perform the legs?

    They execute the legs if the following holds:
    \begin{equation}
        E(A_1+A_2)>E(A).
    \end{equation}
    Let's assume the opportunity occurs on $D_1$ first. This means the inequality is approximately:
    \begin{equation}
        A_1+ A_2 P(A_2|A_1)>A P(A_2) \approx A_1 > (A-A_2)P(A_2).
    \end{equation}
    (This conditional is likely less than $P(A_2)$ as $A_2$ increases given $A_1$).
    Replacing the left by $(A_1+ (e_1+e_2))P(A_2)$, we get:
    \begin{equation}
        A_1(1-P(A_2))>(e_1+e_2)P(A_2).
    \end{equation}
    Include numbers for these values!!!
\end{example}

\subsection{Shared Sequencer Dominance across domains}

Consider a group of validators across multiple domains. These validators agree to offer a service to users along the lines of \textbf{While we are in charge of mining proceeding blocks on 2 or more domains, we will provide a service to include transactions on all controlled domains in the proceeding blocks.}

Splitting an order across multiple domains might reduce the fees received by a DEX. If an order over impacts a single DEX, that DEX will be arbed back in line (back-running the order), while all other DEXs will be arbed to align with the order impact.

\subsection{Questions arising from The Bible}

Is MEV greater across domains?
Yes. Front-runs can be executed at better prices, with less impact when orders are executed on more liquidity (important when direction is informed).
Where (minor) price discrepancies arise across domain, searchers have the option to execute orders on the best liquidity. 

\subsection{$N$ rational sequencers}

Consider two domains where both sequencers understand that shared MEV is greater than independent MEV. Both sequencers can hide the information in their mempools, equivalent to private order-flow. Can we describe a protocol allowing these sequencers to extract the maximal joint MEV? Let's say both sequencers have a shared MEV pricing oracle to price the MEV of a given block. The sequencers then price the joint MEV of the 2 domains, and split the difference between the two domains. In the case of 3 or more domains, most of the joint MEV may be originating from one domain (the domain with the largest order-flow). The marginal contribution of this chain can be computed... (there is work doing this).

A concern with this approach is the difference in confirmation times across domains. If the largest marginal contributor to the joint MEV happens to have the slowest confirmation times, the instantaneous joint MEV at the time of execution of the main contributor might be close to 0, as all other chains have used the information to extract the MEV from their chains already. Furthermore, the marginal contribution of the main chain be removed as soon as the first chain confirms, updating the domain state to reflect the information in the main contributor chain. 

A solution is dividing up the block-space of the slower chains into sub-blocks, aligned with the rate of blocks occurring on the faster chains. For example, let's assume all blockchains in the colluding set of $n$ chains produce blocks at a rate of $2^{r_i}$ per time unit, for some $r_i>0$, with $r_i>r_{i+1}$. This implies all blockchain $i$ needs to create blocks containing $2^{r_i-r_1}$ sub-blocks. This further restricts the contents of these blockchains, as blocks on slower chains must be big enough to allow for these sub-blocks.

For simplicity, let's assume all blockchains confirm blocks at the same time.  Let's further assume that when an order reaches the mempool, there is nothing actionable in continuous time domains (this is equivalent to a producer actioning on all transactional information as soon as it enters the mempool in continuous time domains). 

\begin{enumerate}
   \item Can producers agree on an MEV pricing function?
   \item Is there an incentive to generate fake (marginal) MEV in a chain to increase a player's marginal contribution to the joint MEV? In the 2-chain case, this is protected against because the MEV must be \textit{extractable} on the other chain. Specifically, if a transaction set on one chain adds to the joint MEV between that chain and another, that value is extractable
    \item Should a producer share all information as it enters the pool, or at the end?
    \item a
    \item If a continuous time domain exists, should a producer share that information with another producer before actioning on it in the continuous time domain?
\end{enumerate}

\subsection{SUAVE and Beyond}

SUAVE's goal is to provide a domain where users submit intents which can be executed in any domain, and searchers compete to execute these intents. There is a limit to the effectiveness of this system as the atomicity of cross-domain transactions is only possible if the searcher is able to include all legs of the transaction in each domain. This requires independent auctions to include the transaction in each domain. One suggestion is for domains to sell block building rights in advance, futures style. This requires an anticipation of future value creation and order-flow, which is a centralizing vector. Another could be the instantaneous auctioning of the right to build the current block, with proposers committed to respecting the result of the auction. If this is done in a Dutch Auction style, it may be the 

A simpler set-up might be that cross-domain validators can opt in to a meta-chain where cross-domain orders are atomically committed. This makes less sense as it needs to be the builder of both blocks that accepts the transaction for it to be priced correctly. It is possible that each chain agrees to a certain pricing curve/allocations for transactions to be \textit{guaranteed to execute} in their respective chains if they are included in the meta-chain. A more realistic requirement might be that no other transaction included before that transaction no already in the guaranteed chain invalidates it. This gives users a path to atomic transactions guaranteed by the builder. If the pricing curve for user transactions is increasing (fee escalator), and the curves for guaranteed inclusion are decreasing (or maybe just decreasing while demand remains constant), user transactions should eventually get included. We can add functionalities like a "fee-budget" which allows the user fee to be allocated dynamically to the chains, with higher fees paid to chains costing more at the time, allowing the transaction to be included as soon as the total fee required by the set of chains is equal to the budget specified by the user. 

On a similar vein, users can set a negative fee budget, with the difference between the required sum and fee budget paid by a cross-domain searcher. If the only requirement on these transactions is to not be invalidated, it may be in the interest of a single-/cross-domain searcher to bundle one or more of the legs on the respective domains (as long as the individual leg gets executed, this is fine). This implied rebate from a negative budget is received by the user. 

This guaranteed inclusion fee (curve) set by the block builder should represent the optionality given up by the builder (decreasing in time to the block), plus some buffer to account for the potential difference between demand and the base fee implied by the curve. These meta-transactions practically give the transaction top-of-block rights in the sub-domains, so it is important that the builders are actively updating the top of block state on the meta-chain (with transactions of their own).

This protocol might see a disproportional amount of fees being paid to the slowest chains. This might not be a bad thing, as this higher fee is paying for an earlier commitment guarantee.

This protocol can be coupled with SUAVE to provide instantaneous atomic guarantees at the cross-domain level.

\subsubsection{Design Considerations}

There are several assumptions and requirements of such a system. The main assumption here is that all domains are on-boarded all the time. In reality, only a percentage of proposers/builders on each chain will be on-boarded. This will create many intervals in which the guarantees of the protocol are not atomic. An example of this, is where one domain has a non-participating proposer before a participating proposer who invalidates the leg of a committed cross-domain transaction. To solve this, the protocol needs to be highly synchronized, understanding at all times which domains are accepting transactions. This might be achievable by the set of participating builders sending a multi-sig. to the protocol activating transactions on that set of domains, and specifying the parameters for that auction. The chain needs to opt in to an auction, specifying the number of meta-blocks/timestamp/conditions until transactions are no longer accepted. Are there incentives for validators on the meta-chain to censor builders? I would think not as the system value is strictly increased if more domains opt in to the system, which censorship would disincentivize.

How can the meta-chain enforce inclusion on the sub-domains. The easiest way is forcing the sub-domains to provide regular checkpoints of the meta-chain on the sub-domain. If a transaction is included on the meta-chain, it must be included and executed on the sub-domain. Proving inclusion on the meta-chain and non-inclusion on the sub-domain would suffice. This still may be insufficient to fully disincentivize, so forcing a deposit of tokens on one or more of the other sub-domains and/or meta chain might also be required. Withdrawal of tokens from these contracts requires a withdrawal transaction to be included on the meta chain, and proof on the sub-domain. 

\subsubsection{System Requirements}

One of the most important elements of this system is a requirement for transactions added to the meta-chain to be enforceable. This probably needs some sort of strong synchronicity assumption. The best way to do this would be a heartbeat from active proposers, so without a proposer heartbeat, non-checkpointed transactions (since the last heartbeat) are not enforceable. Participating proposers agree to a minimum heartbeat frequency, which if broken, can lead to social slashing. Providing a heartbeat is equivalent to acknowledging all transactions up to that point have been seen. If one proposer doesn't provide a heartbeat, it only gets seen by other proposers at the next heartbeat, which should be considered by other proposers. 

Does providing a heartbeat amount to a validity check? I think it can. A soft ordering is applied to the meta chain, which must be confirmed by the individual proposers. For this to be possible, there must be some quick validation of state transitions happening at meta-block building time. Having access to the last block should be sufficient to do this, although the producer can choose to invalidate any of the transactions. Incorrect invalidation can be punished by slashing. Can the meta-chain force the builder to obey the ordering of the meta-chain? I guess not, but even social slashing on the meta-chain should be sufficient to prevent repeated misbehaviour. 

\subsubsection*{Roll-ups to avoid congestion}

Domains attached to this shared sequencer would likely come under higher demand, which each domain would need to handle. This might involve some roll-up style compression of gas costs from shared sequencer to main chain. \textbf{Intents might be a nice way to handle this.} Keep the requirements on final state changes, and not on intermediate states.

\subsection{Justifying a Shared Sequencer}

Tweet: Loss-versus-rebalancing (LVR) is not dependent on how delayed the liquidity provider/DEX is. Once there is a delay, the cost is ~constant per unit-time. 
If you're not joint-first, you're last.

Following replies on this, there are simulation results (which I have been assured are provable), which indicate that LVR grows in the square root of block time/delay to the updated information. I think the necessary assumption is modeling volatility/time as close to continuous as possible, with results demonstrating that the price often reverts to a non-arbitrageable state (including fee) over the course of the block time. Proving this analytically is a little tricky... However, this provides strong motivation to be as close to synchronized to other domains as possible.

This is a strong advocation for providing some sort of shared-sequencer to allow all protocols to be attached to the same approximate continuous-time feed. From the latest Millionis paper, "the asymptotic regime analysis above points to a significant potential mitigator of arbitrage profits: running a chain with lower
mean inter-block time (essentially, a faster chain), since we show that this effectively reduces arbitrage profit without negatively impacting LP fee income derived from noise trading"

The important thing will be making it non-binding without signing from the player in control of the domains. 

\subsubsection{Capabilities in a Cross-Domain World}

\begin{enumerate}
    \item Atomic cross-domain orders (All-or-nothing orders). Example: Buy ETH selling USDC up to a price of 2,000 USDC, buying $x$ on domain A, and $(1-x)$ on domain B.
    \item Atomic cross-domain swaps (transactions conditional on previous transactions). Example:  1. Buy ETH selling USDC on domain A, 2. bridge the ETH, 3. buy USDT selling the ETH on domain B. 3 conditional on 2 conditional on 1.
    \item Cross-domain flash loans (related to previous point). Using bridge assets as flash-loan collateral.
    \item Reduced-/0-LVR. All domains are effectively synchronized, meaning prices will update as soon as fees and gas prices allow, as opposed to waiting until block proposing time. 
\end{enumerate}

\subsection{Protocol Description: 2 Domain Case}

Consider producers $P_1, \ P_2$ controlling 2 domains (chains) $C_1, \ C_2$ with block times $T_1, \ T_2$ and a shared sequencer $SS$. This shared sequencer is controlled by a rational player elected\footnote{Elected? This probably requires stake deposits to provide some sort of incentive} by $P_1, \ P_2$. The sequencer accepts both single-domain and cross-domain transactions from a group of MEV searchers who require pre-block confirmation from $P_1$ and $P_2$. $P_1$ and $P_2$ specify a cost-demand curve for this pre-block confirmation service at initialization. Blocks on $SS$ occur every time $t<<T_1,T_2$. For a transaction included in $SS$ at time $t_0$ the block is sent to $P_1$ and $P_2$ for signing. Each $P_i$ responds with a signature on valid transactions. When $SS$ receives the signatures back, $SS$ then bundles the signatures and forwards and signs the set of signatures to each producer. If each transaction involving $b\in \{ 1, 2\}$ domains has $b$ signatures, the transaction in domain $i$ can be included. This signed set of signatures is enough to provide strong economic guarantees. 

What type of equivocations are possible?
\begin{enumerate}
    \item $SS$ sends equivocating signature sets to $P_1$ and $P_2$: Either/both can pass this equivocation to smart contracts on their respective chains to punish $SS$, potentially reimbursing the affected transactions, although burning likely eliminates collusion vectors.
    \item $P_i$ disobeys the signature set received by another player. If $P_i$ goes offline after sending a signature, there needs to be an override ensuring the transactions as per the shared sequencer get executed first. If $P_i$ tries to ignore $SS$
\end{enumerate}

\subsubsection{Requirements of the Shared Sequencer}

The most important part of this system is data availability. A builder only provides a heartbeat at height $H$ if there is a data availability proof for height $H$. Celestia provides a data availability layer. 

\subsection{Uniswap in a cross-domain world}

\begin{enumerate}
    \item Can a cross-domain DEX incentivize the transmission of information to other domains to avoid LVR? 
    \item Can a DEX exist on the meta-system? Probably not if we are using states from asynchronous states.
\end{enumerate}

\subsection{Uniswap Live Trading}

There is an app-specific chain/sequencer which replicates the liquidity of the on-chain liquidity pools. There are several options for this. 

\begin{enumerate}
    \item Participating builders/proposers upload the current state of the pools in their blockchain to the SS, agreeing to process Uniswap transactions executed on the SS in their blockchain. In exchange, the builders get reduced fees in the Uniswap pools in their blockchains. In theory, this incentivizes builders (orders can be executed at reduced app fee, also better for users) and the liquidity providers. If a roll-up of the SS can be applied to capture the live-trading, this captures fees typically lost to LVR. If builders from multiple chains participate, this allows for atomic cross-chain swaps. 
    \item There is a Uniswap chain replicating the liquidity of each chain and pool. Every liquidity token locks half of the assets in an off-chain Uniswap pool. Every block in the normal pools, the Uniswap chain emits a pool update message. If a normal Uniswap pool passes in the pool update message, the fees for that block are reduced. 
    Effectively, the off-chain protocol creates a batch of transactions. Submitting a batch to the blockchain reduces the fees in the on-chain protocol. This creates an incentive for builders to include batches. However, this leaves the Uniswap chain as a point of failure. 
\end{enumerate}

\subsection{Comments}

"We're happy to accept centralizing vectors in certain domains, as long as other domains remain decentralized."

Proposers would play the game with the shared sequencer if blocks in the sequencer were only valid if the set of transactions were (conditionally) valid on each chain (requiring a signature, or set of signatures from validity checkers with low latency who are slasheable), and each set contains a data availability proof providing something like $99.9999\%$ chance, or greater that each proposer can see the relevant transactions the block (this is achievable using data availability sampling, albeit in the 20-40s range). If the proposer does not include the set in his or her block, their stake can be slashed on either/both the SS and the respective chains. If these proofs are strong enough, we can get some nice properties. If blocks are produced at most every 1 second, we would need data availability proofs confirmed before the blocks on participating chain are published.
Such proofs would be acceptable for participating block proposers to be sure the transactions are available to the proposer. 

What is the incentive for proposers? Continued decentralization should be huge. Can they increase their revenue? Participating proposers can set their own fee curves, reflecting the demand and value added by their blockchains.

\subsection{Diamonte}

Orders can have 3 types, rebated, hedged (tokens removed will be fully repaid, and are locked in collateral) (this is in-line with some of the ideas in Osmosis \footnote{\url{https://osmosis.zone/blog/osmosis-protorev-by-skip-protocol-on-chain-app-directed-arbitrage}}, and closing (using collateral tokens).
\section{Preliminaries}

This section introduces the key terminology and definitions needed to understand cross-domain MEV. A possibly more interesting approach for this paper is to increase understanding of cross-domain value extractions opportunities, rather than try to reason about whether these opportunities are maximal

\subsection{Categorizing Cross-Domain Services}

We need more information on bridges. Shared sequencing services like Celestia.

\subsection{Categorizing Cross-Domain Value}

\subsection{Categorizing Cross-Domain Extractable Value}

\subsection{Extracting Cross-Domain MEV}

\subsection{Centralizing the Extraction Process}

Centralization is primarily caused by the need to reduce latency. \url{https://frontier.tech/exploration-of-mev-latencies}.

\subsubsection{Centralized Searchers}

As long as cross-domain opportunities, there will be a requirement for extractors to co-locate on each domain in which the opportunity exists. This is extremely capital intensive, creating a centralizing effect on extractors. 

\subsubsection{Centralized Proposers}

The only way to guarantee the inclusion of $n$ transactions in $n$ individual domains a
is to control the block being proposed. Builders can pay for this right, but at the heart of this control is the proposers. If a certain player proposes $x$ of the blocks on two separate domains with similar block times, $x^2$ of the time the player has full control of cross-domain opportunities. If there is a significant difference in block times, this approaches $x$, as the proposer almost always controls a fast chain block while in control of the slow chain block, meaning every time the proposer controls a slow-chain block, the proposer will be able to extract every cross-domain opportunity.

\subsection{Decentralizing the Extraction Process}

This section discusses the current proposed approaches to facilitate CDEV. 

\subsubsection{Cross-Domain searcher orderflow auctions}

Flashbots' SUAVE is the primary example of this method. SUAVE incentivizes the centralization of both searchers and proposers, as guarantees are less probabilistic. This is in addition to the need for a (potentially centralized) SUAVE chain. 

\subsubsection{Partial block auctions and inclusion lists}

This post from Vitalik describes some high-level ideas for how proposers can enforce specific transaction sets get included by the builder. \url{https://ethresear.ch/t/how-much-can-we-constrain-builders-without-bringing-back-heavy-burdens-to-proposers/13808}.
Is it possible to extend this to a shared sequencer among proposers. Searchers in the shared sequencer submit all-or-nothing bundles to the SS. The users trust the SS to ensure each leg can be executed. HOW? 

Can we make searchers responsible for ensuring validity? One way to do this would be to make each set of transactions selected by one SS builder. The winner gets to send a bundle to each relayer. 

\subsubsection{Decentralizing the Effects of Cross-chain MEV}

Can we construct a shared sequencer that doesn't require searchers with large resource capabilities on multiple domains? It seems impossible to create a cross-domain system without at least low-latency searchers, so at least removing the requirement for control is a positive. The only way to remove an incentive for searchers to try and dominate control, is for control to be credibly auctioned.

\subsubsection{Protocol defences against cross-domain MEV}

Diamond plays an important role here. Diamond allows protocols to capture LVR without centralizing toooo much.

If protocols deploy on multiple chains, they can coordinate to allow some degree of cross-chain communication. Consider two chains where proof of ownership of tokens on one chain can be proven on the other, say for example from LPs in both chains. Such players are allowed to send signals which can be interpreted by both chains. These signals can be used to interact with native chain protocols. For example, a signal from such a player known to be actionable on the other chain if it is invalid can be used to update pool prices and/or fees for the proceeding block. 

Protocols trust an oracle which tracks opted in players with tokens locked on both chains. These players can provide oracle results for other on chain protocols (such as replicated protocols on those other chains). Incorrect oracle updates are then punishable on the other chain. If finality is a risk, this can be reflected in a type of insurance fund that repays these cross-chain players for slashes caused by reorgs. \textbf{Note} if we are only concerned with protocols where leaders cannot equivocate, we can achieve something like this with a need for re-org insurance. It is possible to enforce punishments locally, but after a state update from the other chains have been received. This is likely too late to ensure prices are correct. 

The fees on such protocols can be higher to reflect the value lost to cross domain value extraction. it might also be possible that these players can be responsible for atomic cross chain transactions, although this is less clear. We can probably get closer to probabilistic cross-chain transactions, but guaranteeing atomicity might harm protocol liveness. 

\textbf{What are the advantages of this over Diamond?} In reality the watchers can perform the top of block actions in both chains. The requirement to hold tokens natively is less in this watcher protocol, although requires more trust, depending on the ability to post (ir)regular state updates. x

\subsection{A first attempt to generalize cross-domain MEV}

As identified in \cite{obadia2021unity}, the cross-domain world unlocks interesting paths that do not exist in the single-domain world, such as access to tokens outside of the single domain. Without atomicity, such opportunities are unlikely to dominate. These opportunities are only possible if there is at least one common asset on each chain. We should be able to map everything back to that asset eventually. Specifically, every asset on each chain has a market price which can be translated into the value of any other asset on any domain. 

Given a set of orders for a token, all rational players in the system have approximately the same interpretation of the expect price of the token. Furthermore, all rational players can compute the optimal ordering of these tokens to maximize the profits or arbitrarily many arbitrage trades. Without transaction fees and gas limits, rational players will alway move the price of every asset to the expected price. 

If there is new information on another domain which affects the price, there are two scenarios for a rational player. The player finds the information out before acting on the current domain, or after. 

The expected returns are strictly greater when the player finds the information out before acting on the current domain. This is the primary source of MEV. With a finite set of externally provided transactions which can manipulate the domain, profit is strictly increased by receiving all available information before choosing the best response. As the number of domains increase, so to does the number of interpretable signals that directly affect the price of assets on each chain, which in turn decreases the quality of information in the current domain.  

It could be argued that some MEV is not representable in such a way. Specifically, consider MEV which is not directly accessible by the public. For example, only players in possession of a particular NFT have the ability to access an underpriced set of tokens. I don't think this contradicts the definition. These NFTs have a value equal to the opportunity.

As we increase the number of domains, we decrease the relative signal strength of our own domain. Relative signal strength might be an interesting way to consider MEV.

Furthermore, adding centralized liquidity sources where traders can trade close to instantly, it makes sense that these centralized liquidity sources are close to true reflections of the current best guess for the price of each listed token. Not only do these domains attract signals due to their low latency, they are also the gateway between onboarding and offboarding from the blockchain world. These signals are perhaps the most meaningful when estimating the true value of a token and/or the ecosystem in which it exists. Network effects (REFs) have often been considered one of the value cornerstones for any system, and these network effect signals are greatest at the entry points to the blockchain ecosystem. 

Consider $n$ domains $D_1, ..., D_n$, and the information available on domain $D_i$ described by $I_i$. The information for $D_i$ is only made public when $D_i$ updates, although there are some players who are (partially) aware of $I_i$ before $D_i$ updates (such as winning searchers/builders). We introduce the idea of a perfect DEX $\Phi$, such that the pricing function of $\Phi$, $p_\Phi$ is fully aware of $I_1,..,I_n$. 

Consider $m$ rational players, each with a private view (opinion) of $p_\Phi$, denoted $p_{\Phi,i}$ based on their interpretation of $I_1,...,I_n$. We also assume each player can trade frictionlessly at $p_{\Phi,i}$.

Let us examine the single domain case, which may exist for a small memecoin. Let's start with the single DEX case. If all players have the same mempool, each rational player will have the same interpretation of $p_\Phi$. Given a particular mempool state, each rational player $P_i$ will try to construct a block containing a sequence of personalized trades $T_i=\{t_{i,1},...,t_{i,k}\}$, such that $\sum{\textit{profit}(t_{i,j})}$ is maximized. As the players are rational, it must be that the on-chain price of the token after $t_{i,k}$ is $p_\Phi$. If all orders are routed through the DEX, the DEX does not experience LVR.

Let's now assume a second DEX opens on the same domain, but all non-builder orders are still placed in the original DEX. The builder will always set the price of the second DEX to $p_\Phi$. It seems like the second DEX is paying LVR to the builder. However, if both contracts are public, it is more likely that both DEXs are actually paying LVR to the builders, with the original receiving a larger fee, although unrelated to the LVR being paid.
