# Supplementary material for: SoK: Cross-Domain MEV
Source: arXiv:2308.04159 source file (2023-08-08)
Supplement: Supplementary file 3 [file Resources.tex]

Some research developments in this area are: 
\begin{enumerate}
    
    \item On The Quality Of Cryptocurrency Markets: Centralized Versus Decentralized Exchanges \url{https://arxiv.org/pdf/2112.07386.pdf}.
    \item An Empirical Study of Market Inefficiencies in Uniswap and SushiSwap \url{https://arxiv.org/pdf/2203.07774.pdf}. This paper shows that on-chain markets become efficient, and opporunities disappear.
    \item Blockchain Intra- and Interoperability \url{https://static1.squarespace.com/static/57af6f83893fc027c794e637/t/60d7b9c0e71eb125bdc7928d/1624750530252/32+2021+Lipton+Hardjono+Blockchain+Intra+and+Interoperability.pdf}. This paper tries to formalize the players... Moderately interesting, but not really. 
    \item Unity is Strength: A Formalization of Cross-Domain Maximal Extractable Value \url{https://arxiv.org/pdf/2112.01472.pdf}.
    \item ODOS: DEX/cross-chain??? aggregator. Provides optimal routing across DEXs\url{https://odos.xyz/} Cross Domain Arb tracker: \url{https://www.odos.xyz/arbitrage}.
   
    \item HOP Exchange. Cross shard DEX where the bridge is effectively an AMM with a common token, managed by a \textit{bonder}. This bonder skips the necessity to always communicate via the Layer 1 blockchain, in exchange for a fee. 
    \item deBridge. A cross-chain messaging bridge (including for bridging assets) \url{https://debridge.finance/}.
    \item WooFi: Cross chain DEX using CEX prices as an oracle. 
    \item A lot of protocols are using LayerZero's Stargate to relay messages interchain (at least Sushi and WooFi). The protocol requires a relayer and oracle to verify transactions have been committed on the source chain before executing on the destination chain. No proving is done on the destination chain, making these intermediaries centralized players. 
    \item Hashflow seem to be the largest active cross-chain DEX. Requires active MMs providing quotes for users, presumably owning tokens on both chains. \url{https://docs.hashflow.com/hashflow/product/bridgeless-cross-chain-swaps}.
    \item Chainge Finance appears to offer a cross-chain DEX aggregator, \textit{finding the best price available} \url{https://www.coindesk.com/sponsored-content/cross-chain-liquidity-aggregation-delivers-best-prices-and-unlimited-liquidity/}.
    \item Thorchain offers cross-chain swaps, but all transactions happen on the ThorChain (Cosmos).
    \item Dodo allows for cross-chain swaps, althought seems to involve active quoting. Very unclear where tokens are coming from. (using "decentralized price oracles").
    \item Nice article by Variant Fund  \url{https://variant.fund/articles/cross-chain-order-flow-auctions/}.  Interesting terms: \begin{itemize}
        \item New sources of network effects emerge for L2s, we could see L2s buy up significant portions of L1 blockspace in order to crowd out other L2s’ access.
        \item App layer projects could run builders, with the goal of minimizing fee extraction for users.
    \end{itemize} 
    \item Osmosis ProtoRev. The Osmosis chain seems to be executing cyclic arbitrage (albeit restricted to the osmosis chain). Improving cross-chain atomicity improves the democratization of cross chain MEV.   \url{https://osmosis.zone/blog/osmosis-protorev-by-skip-protocol-on-chain-app-directed-arbitrage}
    \item Volt Capital. Primers on MEV across chains, with some interesting links and thoughts on current directions in the space  \url{https://volt.capital/writing}
    \item Nice article by JCharbonneau on SUAVE \url{https://mirror.xyz/jon-dba.eth/NTg5FSq1o_YiL_KJrKBOsOkyeiNUPobvZUrLBGceagg}. Some highlights:\begin{enumerate}
        \item ...this means that SUAVE cannot guarantee atomic inclusion of X-chain transactions by itself. You need the proposers of respective chains to agree on atomic inclusion for that guarantee to be enforced.
        \item SUAVE can’t provide “technical X-domain atomicity” on its own, but it can provide “economic X-domain atomicity” in this sense from the user perspective (though the executor may get stuck holding the risk, at an increased fee).
    \end{enumerate}
    \item Cross Chain communication is \textbf{impossible} without a TTP \url{https://eprint.iacr.org/2019/1128.pdf}. This paper also does a good job at formalization of cross-chain messaging. 
    \item Thread by @bertcmiller on how holding inventory risk results in strict domination of profits, specifically for sandwiching on Ethereum in this case. I think this is a good advocation that this will be the end goal \url{https://twitter.com/bertcmiller/status/1656392881538744321}.
    \item Mekatech \url{https://meka.tech/zenith} is trying to build a sequencer for multiple blockchains . One of their protections is: \textit{If for any reason Zenith fails to propose a block within a strict time limit, then the code falls back to the normal block production behavior.} These lads also provided an estimate of cross-domain opportunities on Cosmos chains \url{https://meka.tech/writing/analysing-cross-chain-arbitrage-opportunities-for-atom-fee57867-4385-4ead-b19c-8db75a753226}.
    
\end{enumerate}

Uniswap has approximately $5\%$ TVL outside of Ethereum. Several links mention cross-domain MEV as a centralizing force. Validators may be creating blocks on multiple blockchains. What effect will this have? Are there any protocols that are more vulnerable to the effect of multi-chain control?

\subsection{}
