# Supplementary material for: SoK: Cross-Domain MEV
Source: arXiv:2308.04159 source file (2023-08-08)
Supplement: Supplementary file 5 [file PrelimsDraft.tex]

\section{Preliminaries}

This section introduces the key terminology and definitions needed to understand cross-domain MEV. A possibly more interesting approach for this paper is to increase understanding of cross-domain value extractions opportunities, rather than try to reason about whether these opportunities are maximal


\subsection{Categorizing Cross-Domain Services}

We need more information on bridges. Shared sequencing services like Celestia.

\subsection{Categorizing Cross-Domain Value}




\subsection{Categorizing Cross-Domain Extractable Value}


\subsection{Extracting Cross-Domain MEV}

\subsection{Centralizing the Extraction Process}

Centralization is primarily caused by the need to reduce latency. \url{https://frontier.tech/exploration-of-mev-latencies}.

\subsubsection{Centralized Searchers}

As long as cross-domain opportunities, there will be a requirement for extractors to co-locate on each domain in which the opportunity exists. This is extremely capital intensive, creating a centralizing effect on extractors. 

\subsubsection{Centralized Proposers}

The only way to guarantee the inclusion of $n$ transactions in $n$ individual domains a
is to control the block being proposed. Builders can pay for this right, but at the heart of this control is the proposers. If a certain player proposes $x$ of the blocks on two separate domains with similar block times, $x^2$ of the time the player has full control of cross-domain opportunities. If there is a significant difference in block times, this approaches $x$, as the proposer almost always controls a fast chain block while in control of the slow chain block, meaning every time the proposer controls a slow-chain block, the proposer will be able to extract every cross-domain opportunity.

\subsection{Decentralizing the Extraction Process}

This section discusses the current proposed approaches to facilitate CDEV. 

\subsubsection{Cross-Domain searcher orderflow auctions}

Flashbots' SUAVE is the primary example of this method. SUAVE incentivizes the centralization of both searchers and proposers, as guarantees are less probabilistic. This is in addition to the need for a (potentially centralized) SUAVE chain. 

\subsubsection{Partial block auctions and inclusion lists}

This post from Vitalik describes some high-level ideas for how proposers can enforce specific transaction sets get included by the builder. \url{https://ethresear.ch/t/how-much-can-we-constrain-builders-without-bringing-back-heavy-burdens-to-proposers/13808}.
Is it possible to extend this to a shared sequencer among proposers. Searchers in the shared sequencer submit all-or-nothing bundles to the SS. The users trust the SS to ensure each leg can be executed. HOW? 

Can we make searchers responsible for ensuring validity? One way to do this would be to make each set of transactions selected by one SS builder. The winner gets to send a bundle to each relayer. 

\subsubsection{Decentralizing the Effects of Cross-chain MEV}

Can we construct a shared sequencer that doesn't require searchers with large resource capabilities on multiple domains? It seems impossible to create a cross-domain system without at least low-latency searchers, so at least removing the requirement for control is a positive. The only way to remove an incentive for searchers to try and dominate control, is for control to be credibly auctioned.

\subsubsection{Protocol defences against cross-domain MEV}

Diamond plays an important role here. Diamond allows protocols to capture LVR without centralizing toooo much.

If protocols deploy on multiple chains, they can coordinate to allow some degree of cross-chain communication. Consider two chains where proof of ownership of tokens on one chain can be proven on the other, say for example from LPs in both chains. Such players are allowed to send signals which can be interpreted by both chains. These signals can be used to interact with native chain protocols. For example, a signal from such a player known to be actionable on the other chain if it is invalid can be used to update pool prices and/or fees for the proceeding block. 

Protocols trust an oracle which tracks opted in players with tokens locked on both chains. These players can provide oracle results for other on chain protocols (such as replicated protocols on those other chains). Incorrect oracle updates are then punishable on the other chain. If finality is a risk, this can be reflected in a type of insurance fund that repays these cross-chain players for slashes caused by reorgs. \textbf{Note} if we are only concerned with protocols where leaders cannot equivocate, we can achieve something like this with a need for re-org insurance. It is possible to enforce punishments locally, but after a state update from the other chains have been received. This is likely too late to ensure prices are correct. 

The fees on such protocols can be higher to reflect the value lost to cross domain value extraction. it might also be possible that these players can be responsible for atomic cross chain transactions, although this is less clear. We can probably get closer to probabilistic cross-chain transactions, but guaranteeing atomicity might harm protocol liveness. 

\textbf{What are the advantages of this over Diamond?} In reality the watchers can perform the top of block actions in both chains. The requirement to hold tokens natively is less in this watcher protocol, although requires more trust, depending on the ability to post (ir)regular state updates. x

\subsection{A first attempt to generalize cross-domain MEV}

As identified in \cite{obadia2021unity}, the cross-domain world unlocks interesting paths that do not exist in the single-domain world, such as access to tokens outside of the single domain. Without atomicity, such opportunities are unlikely to dominate. These opportunities are only possible if there is at least one common asset on each chain. We should be able to map everything back to that asset eventually. Specifically, every asset on each chain has a market price which can be translated into the value of any other asset on any domain. 

Given a set of orders for a token, all rational players in the system have approximately the same interpretation of the expect price of the token. Furthermore, all rational players can compute the optimal ordering of these tokens to maximize the profits or arbitrarily many arbitrage trades. Without transaction fees and gas limits, rational players will alway move the price of every asset to the expected price. 

If there is new information on another domain which affects the price, there are two scenarios for a rational player. The player finds the information out before acting on the current domain, or after. 

The expected returns are strictly greater when the player finds the information out before acting on the current domain. This is the primary source of MEV. With a finite set of externally provided transactions which can manipulate the domain, profit is strictly increased by receiving all available information before choosing the best response. As the number of domains increase, so to does the number of interpretable signals that directly affect the price of assets on each chain, which in turn decreases the quality of information in the current domain.  

It could be argued that some MEV is not representable in such a way. Specifically, consider MEV which is not directly accessible by the public. For example, only players in possession of a particular NFT have the ability to access an underpriced set of tokens. I don't think this contradicts the definition. These NFTs have a value equal to the opportunity.

As we increase the number of domains, we decrease the relative signal strength of our own domain. Relative signal strength might be an interesting way to consider MEV.

Furthermore, adding centralized liquidity sources where traders can trade close to instantly, it makes sense that these centralized liquidity sources are close to true reflections of the current best guess for the price of each listed token. Not only do these domains attract signals due to their low latency, they are also the gateway between onboarding and offboarding from the blockchain world. These signals are perhaps the most meaningful when estimating the true value of a token and/or the ecosystem in which it exists. Network effects (REFs) have often been considered one of the value cornerstones for any system, and these network effect signals are greatest at the entry points to the blockchain ecosystem. 

Consider $n$ domains $D_1, ..., D_n$, and the information available on domain $D_i$ described by $I_i$. The information for $D_i$ is only made public when $D_i$ updates, although there are some players who are (partially) aware of $I_i$ before $D_i$ updates (such as winning searchers/builders). We introduce the idea of a perfect DEX $\Phi$, such that the pricing function of $\Phi$, $p_\Phi$ is fully aware of $I_1,..,I_n$. 

Consider $m$ rational players, each with a private view (opinion) of $p_\Phi$, denoted $p_{\Phi,i}$ based on their interpretation of $I_1,...,I_n$. We also assume each player can trade frictionlessly at $p_{\Phi,i}$.

Let us examine the single domain case, which may exist for a small memecoin. Let's start with the single DEX case. If all players have the same mempool, each rational player will have the same interpretation of $p_\Phi$. Given a particular mempool state, each rational player $P_i$ will try to construct a block containing a sequence of personalized trades $T_i=\{t_{i,1},...,t_{i,k}\}$, such that $\sum{\textit{profit}(t_{i,j})}$ is maximized. As the players are rational, it must be that the on-chain price of the token after $t_{i,k}$ is $p_\Phi$. If all orders are routed through the DEX, the DEX does not experience LVR.

Let's now assume a second DEX opens on the same domain, but all non-builder orders are still placed in the original DEX. The builder will always set the price of the second DEX to $p_\Phi$. It seems like the second DEX is paying LVR to the builder. However, if both contracts are public, it is more likely that both DEXs are actually paying LVR to the builders, with the original receiving a larger fee, although unrelated to the LVR being paid. 
